# Supplementary material for: A Theoretical Approach for Structuring and Analysing Knowledge Provenance for Visual Analytics
Source: arXiv:2204.00585 source file (2023-10-27)
Supplement: Supplementary file 1 [file appendix.tex]

\bgroup

\begin{table}[htb]
% \vspace{-5mm}%Put here to reduce too much white space after your table
\caption{VAKG's goals compared to the literature.}
\label{tab:comparison}
\begin{center}
\begin{tabular}{ c | m{8em} | l  >{\centering}c  >{\centering}c  >{\centering}c | c c c }

 \hline \multirow{2}{*}{\rotatebox{90}{Area}} & \multirow{2}{*}{Paper} & \multicolumn{4}{ c |}{G1} & \multirow{2}{*}{G2} & \multirow{2}{*}{G3} & \multirow{2}{*}{G4} \\
 \cline{3-6} & & .1 & .2 & .3 & .4 & & & \\
 
 \hline \multicolumn{2}{c|}{VAKG} & X & X & X & X & X & X & X \\ 
 \hline \multirow{8}{*}[-4ex]{\rotatebox{90}{Knowledge model or ontology}} & 
               \citet{sacha2014knowledge}        & X & X & X & X &   &   &   \\ 
 \cline{2-9} & \citet{sacha2018vis4ml}           & X & X & X & X & X &   &   \\ 
 \cline{2-9} & \citet{polowinski2013viso}        & X & X & X & X & X & X &   \\ 
 \cline{2-9} & \citet{von2014interaction}        & X &   & X &   &   & X &   \\ 
 \cline{2-9} & \citet{federico2017role}          & X & X &   & X &   & X &   \\ 
 \cline{2-9} & \citet{brehmer2013multi}          & X & X & X & X & X &   &   \\ 
 \cline{2-9} & \citet{von2019informed}           & X & X &   &   & X &   & X \\ 
 \cline{2-9} & \citet{chen2019ontological}       &   & X & X &   & X & X & X \\
 
  \hline \multirow{5}{*}[0ex]{\rotatebox{90}{Knowledge Graphs}} & 
               \citet{chen2020review}            & X & X & X &   & X & X & X \\ 
 \cline{2-9} & \citet{auer2007dbpedia}           &   & X & X & X & X & X & X \\ 
 \cline{2-9} & \citet{chang2016appgrouper}       &   & X & X &   & X & X & X \\ 
 \cline{2-9} & \citet{he2019aloha}               &   & X & X &   & X & X & X \\ 
 \cline{2-9} & \citet{jin2019recurrent}          & X & X & X & X & X & X & X \\ 
 
  \hline \multirow{3}{*}[0ex]{\rotatebox{90}{Provenance}} & 
               \citet{callahan2006vistrails}     &   &   & X & X &   & X & X \\ 
 \cline{2-9} & \citet{da2009towards}             & X &   & X & X & X &   & X \\ 
 \cline{2-9} & \citet{battle2019characterizing}  & X & X & X & X &   & X &   \\ 
 
  \hline \multirow{5}{*}[0ex]{\rotatebox{90}{Behaviour analysis}} & 
               \citet{heer2008graphical}         &   & X & X &   &   & X & X \\ 
 \cline{2-9} & \citet{clifton2012advanced}       & X & X & X &   &   &   & X \\ 
 \cline{2-9} & \citet{spinner2019explainer}      &   &   & X & X &   & X & X \\ 
 \cline{2-9} & \citet{mathisen2019insideinsights}& X & X &   & X &   & X &   \\ 
 \cline{2-9} & \citet{bernard2017comparing}      & X &   &   & X &   & X & X \\ 
 \hline

\end{tabular}
\end{center}
% \vspace{-25mm}%Put here to reduce too much white space after your table
\end{table}
\egroup

%%%%%%%%%%%%%%%%

\begin{align}
\label{eq:firstknowledge1}
K^T_{t+1} &= P(I)\frac{\partial {K^T}^P}{\partial t} = P(V(D_t, K^\epsilon_{t}, S_t))\frac{\partial {K^T}^P}{\partial t}\\
\label{eq:firstknowledge2}
K^\epsilon_{t+1} &= X(K^T_t)\frac{\partial {K^\epsilon}^X}{\partial t} + A(D_t, S_t, K^\epsilon_t)\frac{\partial {K^T}^A}{\partial t} \\
\label{eq:firstknowledge3}
S_{t+1} &= E(K^T_t)\frac{\partial S^E}{\partial t} + A(D_t, S_t, K^\epsilon_t)\frac{\partial S^A}{\partial t} \\
\label{eq:firstknowledge4}
D_{t+1} &= A(D_t, S_t, K^\epsilon_t)\frac{\partial D^A}{\partial t}
\end{align}
